# Supplementary material for: A Generalizable and Accessible Approach to Machine Learning with Global Satellite Imagery
Source: arXiv:2010.08168 source file (2020-10-16)
Supplement: Supplementary file 2 [file global_to_us_table_v0.tex]

\begin{table}[!ht]
\centering
\begin{tabular}{lccccc}
&&&&& \textbf{Global model} \\
& \textbf{US model}  & \textbf{US model} & \textbf{US model} & \textbf{US model} & \textbf{in US} \\
  & \small{$N$=80,000*}  & \small{$N$=18,414}  & \small{$N$=80,000*}  & \small{$N$=18,414}  & \small{$N^{US}$=18,414}  \\
  \textbf{\textit{Task}} & \small{$K$=8,192} & \small{$K$=8,192}  & \small{$K$=2,048} & \small{$K$=2,048}  & \small{$K$=2,048}  \\
 \hline
&&&&& \\
Forest cover ($R^2$) & 0.91 & 0.90 & 0.88 & 0.88 & 0.67 \\
Elevation ($R^2$)& 0.68 & 0.64 & 0.63 & 0.60 & 0.24 \\
Population density ($R^2$) & 0.73 & 0.72 & 0.69 & 0.69  & 0.48 \\
Nighttime lights ($R^2$) & 0.85& 0.83& 0.82& 0.81& 0.66 \\
&&&&&
\end{tabular}
  \caption{ \textbf{Model performance in the continental US using a model trained within the US versus one trained globally with sparse US data sampling.} 
The main text shows performance with a global model trained on substantially less densely sampled observations ($N^{\text{Global}} = 556,025$; $N^{\text{Global in US}} = 18,414$) and number of features ($K = 2,048$) than in the model trained within the continental US ($N = 80,000$, $K=8,192$). This table compares performance across models trained and tested within the US (columns 1 -- 4) with the model trained on a global sampled and tested on the US (column 5). Column 1 uses the full sample of observations and number of features shown in the main text. Column 2 degrades the sample by limiting $N$, retraining the model within the US using the same number of observations as fall within the US in the sample used to train the global model. Column 3 degrades the sample by limiting $K$, retraining the model within the US using the same number of image features as used to train the global model. Column 4 degrades the sample by limiting both $N$ and $K$, retraining the model within the US using the number of observations and features used to train the global model. Column 5 shows the performance of the global model within the continental US. Each column displays $R^2$ values indicating performance using the optimal hyperparameters after 5-fold cross-validation. Note that the global model relies on substantially poorer data quality than the model trained within the US and that nighttime lights is sampled with population weights in the US model but not in the global model. *$N$=80,000 for all tasks except population density, where $N=73,102$.} \label{tab:globalinUS}
\end{table}
