# Supplementary material for: A Generalizable and Accessible Approach to Machine Learning with Global Satellite Imagery
Source: arXiv:2010.08168 source file (2020-10-16)
Supplement: Supplementary file 3 [file rs_method_comparisons.tex]

There is a growing literature leveraging satellite imagery for global and regional monitoring. Here, we discuss the how our approach fits within this literature, highlighting comparative advantages of different approaches with respect to cost, generalizability, and performance.

One branch of the literature combines pixel-based modelling approaches that leverage expert knowledge and study-specific band-ratios and temporal signatures with computational infrastructure designed for large-scale parallelization to measure outcomes at global scales [e.g. \cite{hansen2013} \cite{Pekel2016a} \cite{Giglio2009a}]. These models tend to be computationally inexpensive – they have relatively few features and simple model architectures – yet they rely on extensive domain expertise and thus their model architectures are not generalizable across outcomes. For example, in Pekel et al 2016’s work to create maps of surface water, “building, testing and validating the expert system took almost two years." These domain-tailored approaches require relatively low compute resources but relatively high domain expertise. For this reason, they do not generalize across domains.

Another class of approach leverages machine learning algorithms, such as neural networks, to learn directly from the data a nonlinear mapping from the satellite image to the outcome [e.g. \cite{Jean2016} \cite{Gechter2018a} \cite{Perez2017}]. These approaches require relatively high compute resources, but relatively low domain expertise. Though the neural network model architecture appears to perform well over many domains, computationally expensive re-training is usually necessary to predict new outcomes. Further, training new models requires expertise in these machine learning methods, access to the imagery data, and large computational resources. 

\methodname\space is distinct from these two methodological clusters, recovering the benefits of the benefits of the more complex machine learning methods without incurring the computational costs and conceptual complexity. As we document below (Section~\ref{sec:cost_analysis}), it is substantially less computationally costly to train, test, and deploy \methodname\space than a commonly used neural network (ResNet18) to monitor more than one domain. Further, \methodname\space requires less domain-knowledge and research time to use than boutique pixel-based methods.
It is the only approach that enables researchers to achieve state of the art performance without access to large-scale computational resources and machine learning expertise or to extensive domain knowledge and abundant time.
%and less machine learning knowledge than neural networks. 
%One would need to monitor many domains, however, for the computational costs of bespoke pixel-based methods such as in \cite{hansen2013} or \cite{Pekel2016a} to exceed that of \methodname\space \todovaishaal{[Calculate this to make sure it’s true]}. We note however, that the bulk of the computation for \methodname\space is domain-agnostic and thus could be executed centrally by a satellite data provider (see Section~\ref{sec:API}).

\paragraph{\textbf{Comparisons to other semi-automated remote sensing pipelines}} 

There is a long literature that seeks to simplify and democratize remote sensing through open source libraries [e.g. \cite{Clewley2014}] and processing chains [e.g. \cite{Inglada2017} \cite{Grippa2017}]. Our approach differs from these in a few important ways. First, we leverage fine resolution imagery and state of the art computer vision algorithms, which enable us to predict a range of variables--including economic variables which are traditionally difficult to measure from space such as income and house value. A recent classification pipeline, for example, struggled to differentiate sub-classes of urban land use due likely to their large pixel size (30m) and relatively small feature set \cite{Inglada2017}. Second, the vast majority of pipelines focus on classification, whereas \methodname\ is designed for regression. In this way, it complements the growing set of land use and land cover products that are being produced. Finally, \methodname\ is designed to achieve high predictive performance across many domains in a computationally efficient way, which to our knowledge has not yet been achieved in the literature. Importantly, the bulk of the computation can be done in a centralized manner and then end-users need only to train models on the tabular data -- this places \methodname\ at a gap in the literature between open source libraries that help users form models starting with the raw imagery, such as \cite{Clewley2014}, and operational remote sensing projects such as \cite{Inglada2017} which observes outcomes directly because \methodname\ enables users to directly.

\todomisc{Add another sentence on transfer of costs from computation}
