# Supplementary material for: A Generalizable and Accessible Approach to Machine Learning with Global Satellite Imagery
Source: arXiv:2010.08168 source file (2020-10-16)
Supplement: Supplementary file 6 [file test_acc_ours_resnet_table.tex]

\begin{table}[!h]
\centering
\begin{tabular}{lcc}
\hline
     & \textbf{Resnet} & \textbf{Random Features} \\
\textbf{Task}       & $R^2$ & $R^2$ \\
\hline  \\
Forest cover    & 0.88                 & 0.90                          \\ 
Elevation     & 0.64                   & 0.67                            \\ 
Population density  & 0.69                   & 0.67                           \\ 
Nighttime lights   & 0.83                 & 0.84                          \\ 
Income        & 0.39                   & 0.41                            \\ 
Road length         & 0.47                   & 0.52                            \\
Housing price  & 0.31                 & 0.39                          \\ 
 \hlinel
\end{tabular}
\caption{\textbf{A comparison of test accuracy between a Resnet and \methodname.} VAISHAAL TO UPDATE this table and add brief details of how each column was constructed in this caption. }
\label{table:cnn_comparison_table}
\end{table}
